# Supplementary material for: Tight bounds for maximum $\ell_1$-margin classifiers
Source: arXiv:2212.03783 source file (2023-01-20)
Supplement: Supplementary file 2 [file appendix.tex]

\documentclass[twoside]{article}

\usepackage{aistats2023}
% If your paper is accepted, change the options for the package
% aistats2022 as follows:
%
%\usepackage[accepted]{aistats2022}
%
% This option will print headings for the title of your paper and
% headings for the authors names, plus a copyright note at the end of
% the first column of the first page.

% If you set papersize explicitly, activate the following three lines:

\setlength{\pdfpageheight}{11in}
\setlength{\pdfpagewidth}{8.5in}

% If you use natbib package, activate the following three lines:
\usepackage[round]{natbib}

% If you use BibTeX in apalike style, activate the following line:
\bibliographystyle{apalike}

\begin{document}

% If your paper is accepted and the title of your paper is very long,
% the style will print as headings an error message. Use the following
% command to supply a shorter title of your paper so that it can be
% used as headings.
%
%\runningtitle{I use this title instead because the last one was very long}

% If your paper is accepted and the number of authors is large, the
% style will print as headings an error message. Use the following
% command to supply a shorter version of the authors names so that
% they can be used as headings (for example, use only the surnames)
%
%\runningauthor{Surname 1, Surname 2, Surname 3, ...., Surname n}

% Supplementary material: To improve readability, you must use a single-column format for the supplementary material.
\ifaistats
\onecolumn
\aistatstitle{Supplementary Material:\\ Tight bounds for maximum $\ell_1$-margin classifiers}
\fi

\subfile{../sections/subsections_theory/step_tools}

\subfile{../sections/subsections_theory/proof_thm2}
\subfile{../sections/subsections_theory/noiseless/sloc_proof}
\subfile{../sections/subsections_theory/noiseless/sunicon_proof}

% \subfile{sectionsAISTATS/proof1_sketch}
\subfile{../sections/subsections_theory/proof_thm1}

\section{Technical Lemmas}
\subfile{../sections/technical_lemmas/TL0_CGMT}
\subfile{../sections/technical_lemmas/TL4_noiseless}
\subfile{../sections/technical_lemmas/TL1_quadratic_bound_fn}
\subfile{../sections/technical_lemmas/TL2_quadratic_plus_fstar_bound}
\subfile{../sections/technical_lemmas/TL3_uniform_convergence_fn}
\subfile{../sections/technical_lemmas/TL5_additional_technical_lemmas}

% \subfile{../sections/subsections_theory/noiseless/sloc_proof}
% \subfile{../sections/subsections_theory/noiseless/sunicon_proof}

\end{document}
